# Supplementary material for: Learned D-AMP: Principled Neural Network based Compressive Image Recovery
Source: arXiv:1704.06625 source file (2017-11-06)
Supplement: Supplementary file 1 [file AppendixTuning.tex]

%This eats up too much space so I cut it

\appendix
\subsection{Proof of Proposition \ref{lem:tuning}}\label{app:tuningproof}

Below is all copied directly from D-AMP paper:

D-AMP can employ any of these tuning schemes. However, once we use a denoising algorithm in the D-AMP framework the problem of tuning the free parameters  of the denoiser seems to become dramatically more difficult: to produce good performance from D-AMP the parameters must be tuned jointly across different iterations. 
 To state this challenge we overload our notation of a denoiser to $D_{\sigma, \tau}$, where $\tau$ denotes the denoiser's parameters. According to this notation the state evolution is given by
\[
o^{l+1}(\tau^0, \tau^1, \ldots, \tau^{l}) = \frac{1}{n}  \mathbb{E} \|D_{\sigma^l, \tau^l} (x_o + \sigma^l \epsilon) -x_o \|_2^2, 
\]
where $(\sigma^l)^2= \frac{o^{l}(\tau^0, \tau^1, \ldots, \tau^{l-1})}{\delta} + \sigma_w^2$. 
Note that we have changed our notation for the state evolution variables to emphasize the dependence of $o^{l+1}$ on the choice of the parameters we pick at at the previous iterations. The first question that we ask is the following: What does the optimality of $\tau^0, \tau^1, \ldots, \tau^l$ mean? Suppose that the sequence of parameters $\tau^l$ is bounded. 

\begin{definition}
A sequence of parameters $\tau_*^1, \ldots, \tau_*^l$ is called optimal at iteration $t+1$ if
\[
o^{l+1}(\tau_*^0, \ldots, \tau_*^l) = \min_{\tau^0, \tau^1, \ldots, \tau^l} o^{l+1}(\tau^0, \tau^1, \ldots, \tau^l).
\]
\end{definition}

Note that $\tau_*^0, \ldots, \tau_*^l$ is optimal in the sense that they produce the smallest mean square error D-AMP can achieve after $t$ iterations. This definition was first given in \cite{MousaviMB13a} for the AMP algorithm based on soft-thresholding. \\

It seems from our formulation that we should solve a joint optimization on $\tau^0, \ldots, \tau^l$ to obtain the optimal values of these parameters. However, it turns out that in D-AMP the optimal parameters can be found much more easily. Consider the following greedy algorithm for setting the parameters: 
\begin{enumerate}[(i)]
\item Tune $\tau^0$ such that $o^{1}(\tau^0)$ is minimized. Call the optimal value $\tau_*^0$. 
\item If $\tau^0, \ldots, \tau^{l-1}$ are set to $\tau^0_*, \ldots, \tau^{l-1}_{*}$, then set $\tau^{l}$ such that it minimizes $o^{l+1}(\tau_*^0, \ldots,\tau^{l-1}_{*}, \tau^l)$. 
\end{enumerate}

Note that the above strategy is a greedy parameter selection. % Furthermore, this optimization is similar to the optimization of the parameters in the denoising literature.
The following result proves that in the context of D-AMP this greedy strategy is optimal:

\begin{lemma}\label{lem:tuning}
Suppose that the denoiser $D_{\sigma, \tau}$ is monotone in the sense that $\inf_\tau \mathbb{E} \|D_{\sigma, \tau} (x_o + \sigma \epsilon) -x_o \|_2^2$ is a non-decreasing function of $\sigma$. If $\tau_*^0, \ldots, \tau_*^l$ is generated according to the greedy tuning algorithm described above, then
\[
o^{l+1}(\tau_*^0, \ldots, \tau_*^l)  \leq o^{l+1}(\tau^0, \ldots, \tau^l), \ \ \forall \tau^0, \ldots, \tau^l, 
\]
for every $t$. 
\end{lemma}

\begin{proof}

Our proof is based on an induction. According to the first step of our procedure we know that 
 \[
 o^1(\tau_*^0) \leq o^1(\tau^0), \ \ \ \ \forall \tau^0.
 \]
 Now suppose that the claim of the theorem is true for every $t \leq T$. We would like to prove that  the result also holds for $t=T+1$, i.e.,
 \[
o^{T+1}(\tau_*^0, \ldots, \tau_*^{T})  \leq o^{T+1}(\tau^0, \ldots, \tau^{T}), \ \ \forall \tau^0, \ldots, \tau^{T}. 
\]
Suppose that it is not true and for $\tau_o^0, \ldots, \tau_o^{T}$ we have
 \begin{equation}\label{eq:contradiction1}
o^{T+1}(\tau_*^0, \ldots, \tau_*^{T})  > o^{T+1}(\tau_o^0, \ldots, \tau_o^{T}). 
\end{equation}
Clearly, 
\[
o^{T+1}(\tau_*^1, \tau_*^2, \ldots, \tau_*^{T}) = \frac{1}{n}  \mathbb{E} \|D_{\sigma^t, \tau^T} (x_o + \sigma_*^{T} \epsilon) -x_o \|_2^2, 
\]
where $ (\sigma_*^T)^2 = \frac{o^{T}(\tau_*^0, \ldots, \tau_*^{T-1})}{\delta} + \sigma_w^2$. If we define $(\sigma_o^T)^2 = \frac{o^{T}(\tau_o^0, \ldots, \tau_o^{T-1})}{\delta} + \sigma_W^2$, then according to the induction assumption $\sigma_*^{T} \leq \sigma_o^T$. Therefore, according to the monotonicity of the denoiser
\begin{eqnarray}
o^{T+1}(\tau_*^0, \tau_*^1, \ldots, \tau_*^{T}) &=& \inf_{\tau^T}\frac{1}{n}  \mathbb{E} \|D_{\sigma_*^T, \tau^T} (x_o + \sigma_*^{T} \epsilon) -x_o \|_2^2 \nonumber\\
&\leq& \inf_{\tau^T}  \frac{1}{n}  \mathbb{E} \|D_{\sigma_o^t, \tau^T} (x_o + \sigma_o^{T} \epsilon) -x_o \|_2^2 \nonumber \\
&\leq& \frac{1}{n}  \mathbb{E} \|D_{\sigma_o^t, \tau_o^T} (x_o + \sigma_o^{T} \epsilon) -x_o \|_2^2 \nonumber \\
&= &o^{T+1}(\tau_o^0, \tau_o^1, \ldots, \tau_o^{T}).  \nonumber
\end{eqnarray}
This is in contradiction with \eqref{eq:contradiction1}. Hence, 
 \[
o^{T+1}(\tau_*^0, \ldots, \tau_*^{T})  \leq o^{T+1}(\tau^0, \ldots, \tau^{T}), \ \ \forall \tau^0, \ldots, \tau^{T}. 
\]
\end{proof}
